# Supplementary material for: DiMSUM: Diffusion Mamba -- A Scalable and Unified Spatial-Frequency Method for Image Generation
Source: arXiv:2411.04168 source file (2025-04-10)
Supplement: Supplementary file 1 [file supp_inference_speed.tex]

\begin{table}
% \begin{wraptable}{r}{0.5\textwidth}
\centering
\small
\vspace{2mm}
\caption{Inference speed comparison between DiT-L/2 and our model to generate one $256\times256$ image, tested on NVIDIA A100 40GB GPU.}
\begin{tabular}{lcr}
 \toprule
Order\textbf{}  & \textbf{Latency} & \textbf{Params} \\ \midrule
DiT-L/2    & 3.8s             & 458M             \\
DiMSUM-L/2 & \textbf{2.2s}             & 460M \\
\bottomrule
\end{tabular}
\vspace{2mm}
\label{tab:supp_scanning_abinference_speed}
\end{table}
% \end{wraptable}
