# Supplementary material for: DiMSUM: Diffusion Mamba -- A Scalable and Unified Spatial-Frequency Method for Image Generation
Source: arXiv:2411.04168 source file (2025-04-10)
Supplement: Supplementary file 2 [file supp_ode_vs_ddpm_solver.tex]

\begin{table}

\centering
\small
    \begin{tabular}{l c c}
        \toprule
         & dopri5 & Euler/DDIM (250NFE) \\
        \midrule
        % \multicolumn{5}{c}{\textbf{CelebA-HQ 512}} \\
        % \midrule
        CelebA 256 & 4.62 & 4.65 \\
        Church 256 & 3.76 & 3.77 \\
        ImageNet 256-G & 2.11 & 2.12 \\
        \bottomrule
    \end{tabular}
    \vspace{3mm}
    \caption{FID50K of ODE solver and DDPM/DDIM solver on CelebA.}
    \label{tab:solver_comp}
\end{table}
