# Supplementary material for: DiMSUM: Diffusion Mamba -- A Scalable and Unified Spatial-Frequency Method for Image Generation
Source: arXiv:2411.04168 source file (2025-04-10)
Supplement: Supplementary file 3 [file supp_gflops.tex]

\begin{table}
\centering
\small
\caption{Speed and GFLOPs comparison. Single-sample generation was performed, and all tests were conducted on an NVIDIA A100 40GB GPU.}
\vspace{2mm}
\begin{tabular}{lcccc}
\toprule
Method &	Time	& MEM & Params &	GFlops \\
\midrule
\multicolumn{5}{c}{256 (latent size: 
$32\times 32$)} \\
\midrule
Ours-L/2 &	2.20s	& 2.42G & 460M &	84.49 \\
DiT-L/2	& 3.80s & 2.30G	& 458M	& 80.74 \\
\midrule
\multicolumn{5}{c}{512 (latent size: 
$64\times 64$)} \\
\midrule
Ours-L/2	& 2.86s & 2.46G &	461M &	337.48 \\
DiT-L/2	& 4.78s & 2.34G &	459M &	361.14 \\
\bottomrule
\end{tabular}
\vspace{2mm}
\label{tab:supp_speed_gflops}
\end{table}
