# Supplementary material for: DiMSUM: Diffusion Mamba -- A Scalable and Unified Spatial-Frequency Method for Image Generation
Source: arXiv:2411.04168 source file (2025-04-10)
Supplement: Supplementary file 4 [file supp_lsun.tex]

\begin{table}[t]
\small
\centering
\vspace{2mm}
\caption{Scaling DiMSUM's parameters on LSUN Church.}
\label{tab:supp_lsun}
\begin{tabular}{lccc}
\toprule
\textbf{Model} & \textbf{FID$\downarrow$} & \textbf{Epochs} & \multicolumn{1}{l}{\textbf{Params}} \\ \hline
DiMSUM-L/2                          & 3.76 & 395 & 460M \\
DiMSUM-XL/2                         & \textbf{3.45}          & 340 & 718M \\
DIFFUSSM    & 3.94          & -   & 673M \\ \hline
StyleGAN     & 4.21          & -   & -    \\
StyleGAN2 & 3.86          & 13K & -    \\ \bottomrule
\end{tabular}
\end{table}
