# Supplementary material for: DiMSUM: Diffusion Mamba -- A Scalable and Unified Spatial-Frequency Method for Image Generation
Source: arXiv:2411.04168 source file (2025-04-10)
Supplement: Supplementary file 5 [file supp_scanning_ab.tex]

\begin{table}
\centering
\small
\caption{Additional ablation of scanning orders involves using window scanning for wavelet blocks and examining the sensitivity of DiMSUM to different scanning orders for spatial blocks. For simplicity, no shared-transformer block is used.}
\vspace{2mm}
\begin{tabular}{lcc}
 \toprule
Order & freq + spatial &spatial \\ \midrule
Bi & 5.47 & 6.39\\
Jpeg & 5.74 &6.26\\
sweep-8& 5.23&5.53 \\
zigma-8& 5.71&6.26 \\
sweep-4 & \textbf{4.92}&5.28 \\
\bottomrule
\end{tabular}
\vspace{2mm}
\label{tab:supp_scanning_ab}
\end{table}
